# Supplementary material for: COMMAND: Certifiable Open Measurable Mandates
Source: arXiv:2203.05015 source file (2022-03-09)
Supplement: Supplementary file 1 [file appendix_b.tex]

\appendix{Addressing Insecurity through Mandates}

% Let's first look at what we identify to be the four causes of insecurity:

Before discussing the details of specific mandates, we find it useful to first identify the sources of insecurity in today's computer systems. We identify four main sources:

\begin{enumerate}
    \item Improper usage---The system is not used properly, often due to user incompetence or ignorance. Examples include users downloading files and running code from untrusted parties or falling victim to other kinds social engineering scams.
    %  This source of insecurity has few technical solutions.
    \item Poor configuration---The system is not configured properly. This can manifest as bad firewall configurations in an otherwise secure router, or using an insecure mode of encryption (e.g. ECB mode) with an otherwise secure block cipher.
    \item Insecure implementation---The system's security features are flawed or easily bypassed. Examples include cryptographic algorithms with timing side channels which can be used to leak secret keys.
    \item Incomplete design---The system is designed without regards to security. Examples include the electric grid and internet (which were both designed for reliability rather than security) and IoT devices, which often have no access restrictions at all.
\end{enumerate}

% \subsection{Tyler Moore's Mandates}

% \subsection{Types of Mandates}

A central planner wishing to improve security can therefore address the root sources of insecurity by issuing mandates to correct the failings in the security marketplace. We discuss nine different types of mandates, each of which are either fairly obvious or have been proposed before. We find that all nine mandates could improve security, but none are sufficient. Additionally, many have serious issues of practicality.

\begin{itemize}
    \item \textit{Mandatory Security Literacy}---To address improper usage, a central planner could require users of a system to pass a mandatory security literacy exam, which would ensure that users can maintain a certain standard of behavior when using computer systems; Such a mandate would be akin to the mandate that automobile drivers must pass a driver's license test before being allowed to drive on public roads. While this mandate would likely improve overall security, many would object to its authoritarian nature. Perhaps a less heavy-handed alternative would be to incentive users to adhere to widely-accepted security practices, such as by offering tax deductions to companies or individuals who use antivirus products or complete educational courses on how to follow best-known security practices. Regardless, the trouble with mandates on user behavior is that even perfect usage does not guarantee freedom against attacks---as long as there is insecurity in the configuration, implementation, or design, no system has any an chance of being secure.
    
    \item \textit{Mandatory Professional Certification}---This mandate is similar to Mandatory Security Literacy, but is aimed at fixing issues in the implementation and configuration of systems rather than regulate end user behavior. The idea is to require that designers of systems be well-educated and well-versed in best security practices. System designers would then need to qualify to practice their profession by demonstrating proficiency in their domain. Such is already the case in many other professions, including medicine and law. This mandate could apply anywhere in the range from the system administrator to the hardware architect. Unlike other professions, the ever-changing domain of computer security would likely require that proficiency tests are recurring, rather than one-time. This mandate would help fix insecure implementations and configurations, but falsely assumes that reasons for insecurity reduce to the decisions of individuals. For example, it doesn't matter how well-versed in security the engineers on a given project are if the design specification eschews all security features in favor of higher performance.
    
    \item \textit{Mandatory Budget Expenditures}---This mandate requires that companies and organizations dedicate a percentage of their operating budget towards security. In some domains this mandate could work particularly well, particularly in services industries (like banks or cloud services providers) where companies are entrusted to maintain the privacy of sensitive customer information. However, in industries that sell goods (like processors and software), mandatory security spending does not guarantee or even necessarily correlate with the security of the end product. For example, a processor company could spend their security budget identifying vulnerabilities in their product, yet ultimately decide that fixing the vulnerabilities would come at the cost of performance, making their product less competitive in the (informationally asymmetric) marketplace.
    
    \item \textit{Mandatory Design Review}---To address insecure implementations, a central planner could require that all system designs (hardware or software) be subject to an external review to identify design vulnerabilities before they can be marketed and sold. In this way, computer products could be certified as ``safe'' to use, in the same way that the U.S. FDA certifies that certain foods and drugs are safe to consume. One obvious issue with this approach is the massive loss of privacy that occurs---companies would lose control over their intellectual property, for example. Another problem is that the external review process would inevitably slow down the pace of technology and become a tar pit of bureaucracy. Finally, while this approach may force companies to identify and perhaps even fix the known vulnerabilities in their products, the mandate suffers from the same issue as the Mandatory Budget Expenditures: Even if companies are shown their products' vulnerabilities, it is unclear how much ``effort'' needs to be dedicated towards fixing the vulnerabilities. In fact, it is unreasonable to suggest that all known vulnerabilities must be fixed. For example, consider the scenario where mandatory external design review discovers a vulnerability in processor (even if the possible exploit is extremely unlikely to happen) and the only known fix is to cut performance in half. Is it reasonable to require that the processor must address the vulnerability? Likely not.
    
    \item \textit{Mandatory Penetration Testing}---This mandate in similar to Mandatory Design Reviews, but has certain advantages. If black-box (rather than white-box) penetration testing is used, then companies can still maintain some privacy, although this is questionable given a sufficiently capable penetration tester. Another advantage is that this approach tests systems as they are being used rather than how they were designed, meaning the mandate addresses both the implementation and configuration causes of insecurity. But despite the advantages, this approach has the same pitfalls as Mandatory Design Reviews, namely that it doesn't tell companies how hard they must try to fix any discovered vulnerabilities.
    
    \item \textit{Harsher Punishments for Insecurity}---Unlike the other preemptive approaches towards mandated security, a central planner could also consider reactive approaches, such as increasing punishments or fines for insecurity, such as when a data breach occurs or a product is found to have an exploitable vulnerability. (Cite Equifax as an example of this. Didn't have time to flesh this out yet.) Such an approach has the benefit of being more \textit{laissez-faire}: Companies are free to determine how and where to best allocate resources to ensure enough security to avoid fines. However, the approach has two major issues: First, there is the perverse incentive for companies to avoid disclosing known issues out of fear of punishment; the end result would likely be that the security of goods and service providers becomes even more opaque. Second, assigning proper attribution would become very difficult if not impossible. 
    % If a software company suffers from a data breach because their product opened up a vulnerability in an open-source library, who's to blame? 
    Consider the case where a software company needs a hardware-based defense to secure their product, but no hardware vendor is willing to include the defense (because of market forces discussed earlier). If the software company's product is exploited, who's fault is it? More generally speaking, it is hard to attribute blame to a company that must rely on products designed without security in mind.
    
    \item \textit{Catch the Criminals}---Rather than mandating the actions of system designers or users, a government could also increase its ability to catch the criminals. In fact, the fact that many cybercriminals act with near-complete impunity is perhaps the core problem behind cybersecurity today \cite{anderson2019measuring}. However, at the present, there are no realistic solutions to this problem available---the best known solution is essentially to monitor the online actions of all users at all times, which is a massive violation of privacy.
    
    \item \textit{Mandatory Security Insurance}---Another reasonable approach could be mandatory security insurance. The basic idea would be to require companies to insure their assets against the threat of cyber attacks. This principle behind this approach is harm reduction, and overall companies might suffer less when insured. However, insurance is also known a moral hazard, where customers might behave more carelessly than they otherwise would have without the insurance. In addition, insurance does not actually address the underlying causes of insecurity, and so overall security does not improve. When we consider that security is largely a community property, any benefits of insurance are therefore suboptimal \cite{grossklags2008secure}. Furthermore, security insurance does not incentivize producers to make goods with security built in, since the producers ultimately aren't the ones who suffer the consequences of insecure products.
    
    \item \textit{Mandatory Standards Compliance}---To address poor configuration, a central planner could require that systems and organizations adhere to a standard. Such is nearly the case with the NIST Cybersecurity Framework \cite{nist}, although this standard is merely a recommendation and not a requirement. While such a mandate may be  a necessary step towards greater security, it is not sufficient: As with the other discussed mandates, it doesn't address the problem of incomplete designs.
    
\end{itemize}

(TODO : what about mandatory design compliance? To fix incomplete designs...)

% Each of these nine discussed mandates would provide benefits
% But none of them cover incomplete design/architectures
% And since security is a full system property, we can't  be secure unless each of the causes of insecurity is addressed.
% We need a tenth mandate that can address this problem...

Of the nine aforementioned mandates, one of them (Catching the Criminals) aims to completely remove the threat of cyberattacks altogether. However, this mandate is generally unrealistic, and we see no way of it being implemented anytime soon. Of the eight remaining mandates, all address at least one of the four identified causes of insecurity, and could be reasonably presented as an approach towards greater security. \footnote{We stress that we do not comment on the relative efficacy, legality, or morality of such mandates, but merely point out that they exist and could plausibly be advanced by a government.} However, while the mandates cover improper usage, improper configuration, and insecure implementation, no mandate present thus far addresses the issue of insecurity by design. That is, none of the above mandates can compensate for any system designed without security in mind. This is because security is thought of as a \textit{full-system property}: All aspects of the system, from hardware to software to configuration to operation, must be secure for a system to be secure. In other words, all four identified sources of insecurity must be addressed to achieve security. Then any government wishing to improve security through market interventions must consider ways to incentivize or mandate that systems be built with security as a first-order design constraint.

\section{Energy as a Mandate}

% We identify features of a mandate that would improve security:
In our search for an appropriate design-level mandate, we first identify some key properties of a good mandate:

\begin{itemize}
    \item A good mandate shouldn't constrain innovation. That is, a good mandate shouldn't cause companies to lose their technological edge over foreign competitors.
    \item A good mandate shouldn't be unreasonably burdensome. Particularly, a good mandate shouldn't disproportionately disadvantage users and small businesses.
    \item A good mandate should be enforceable. A government should be able to tell, without excessive effort, whether or not a mandate is being followed.
    \item The benefits of a good mandate should measurably outweigh the costs.
\end{itemize}

% We can also consider what an ideal hardware security mandate would be:

% \begin{itemize}
%     \item Should cover product lifecylce
%     \item Should cover recurring and non-recurring costs
%     \item Should include clear communication of security benefits
% \end{itemize}

% TODO where were we going with this?

% In addition to these general principles, we can also consider some guidelines more specific to computer system security and, in particular, incentivizing secure designs. First, a good mandate should encompass a product's lifecycle, from development to system integration. The reason for this is so that neither party can shirk on their requirment to be secure: Designers must include features that allow users to be more secure, and users must actually use the features the designers provide.

% Second, a good mandate should cover recurring and 
