# Supplementary material for: COMMAND: Certifiable Open Measurable Mandates
Source: arXiv:2203.05015 source file (2022-03-09)
Supplement: Supplementary file 2 [file appendix_a.tex]

\section{Appendix A}

(Table of HPC events go here)
